# Supplementary material for: 3D-CLFusion: Fast Text-to-3D Rendering with Contrastive Latent Diffusion
Source: arXiv:2303.11938 source file (2023-12-20)
Supplement: Supplementary file 1 [file appendix_old.tex]

\section{More details of datasets and settings}

\paragraph{FFHQ} The FFHQ~\cite{karras2019style} dataset contains 70,000 face images. It is only used for training the initial checkpoint for the generator ($\mathbf{G}$) and the encoders in our framework.

\paragraph{CelebA-HQ} CelebA-HQ~\cite{karras2017progressive,liu2015deep} contains 24,183 training face images and 2,824 testing images. For a fair comparison with previous inversion methods, we only use the test split 2,824 images for testing. In this paper, since all of the testing images from this dataset are from the real human face, we did not present the qualitative visualizations for privacy protection. We only present the quantitative comparisons in the paper.

\paragraph{StyleGAN2-Fake} In order to present the rendering results qualitatively without using real faces, we use the fake yet very realistic faces released by \cite{Karras2019stylegan2}. This dataset contains 263 images of resolution 1,024×1,024 of very realistic human faces generated by StyleGAN2~\cite{Karras2019stylegan2}. We present the testing results qualitatively using these images.

\paragraph{AFHQ} Besides the experiments of inversion on human faces, we also conduct the experiments on animal faces using AFHQ~\cite{choi2020starganv2} and present the results later in the appendix. This dataset contains 15,000 high-quality images at 512×512 resolution and includes three categories of animals which are cats, dogs, and wildlife. Each category has about 5000 images. For each category, the dataset split around 500 images as a test set and provide all remaining images as a training set.


\section{Implementation Details}
% \begin{figure*}[t!]
%   \centering
%   \includegraphics[width=0.9\linewidth]{fig/novel.pdf}
%   \vspace{-5mm}
%   \caption{\textbf{Qualitative comparisons on novel-view rendering.} All of the output images are rendered using face yaw angle $-35^\circ$ degree.}
%   \label{fig:novel}
% %   \vspace{-4mm}
% \end{figure*}
% \input{exp/quant_novel}

All training and testing images are resized to size $256 \times 256 \times 3$, denoting width, height, and channel respectively. The experimental style-based NeRF generator ($G$) employs the checkpoint of StyleNeRF~\cite{gu2021stylenerf} with dimension $256$. The base encoder $E_{base}$ employs a series of residual blocks and 1 linear projection layer. The residual encoder $E_{res}$ employs the architecture from pSp~\cite{richardson2021encoding} and we set the number of residual iterations as 3 in the experiments. We set the dimension of the latent code $w$ as 512 which is the same as the generator and the number of latent code of $w+$ as $17$ following the checkpoint from StyleNeRF~\cite{gu2021stylenerf}.
For the hyperparameter for all of the loss functions, all of losses are equally weighted ($\lambda_{feat}^{base}=1.0$, $\lambda_{img}^{base}=1.0$, $\lambda_{feat}^{res}=1.0$ and $\lambda_{img}^{res}=1.0$) for all the experiments. The batch size is set as $32$ where $16$ is for synthesized images and $16$ is for real images. In the $16$ synthesized images in each batch, we sample $4$ identity latent $w_{syn}$ from StyleNeRF~\cite{gu2021stylenerf} and each $w_{syn}$ samples $4$ camera poses (randomly and uniformly sample yaw angle in the range $-35^{\circ}$ to $+35^{\circ}$ and roll angle as $0$ for simplicity), which can be formulated into these $16$ synthesized images.  We optimize the network using Adam optimizer with the learning rate set as $0.0001$.
Each experiment is conducted on 1 Nvidia GPU A100 (80G) with a batch size of 32 and implemented in PyTorch. We now present more details about the model architecture below:

\paragraph{Generator (StyleNeRF)}
\begin{figure}[t]
  \centering
  \includegraphics[width=\linewidth]{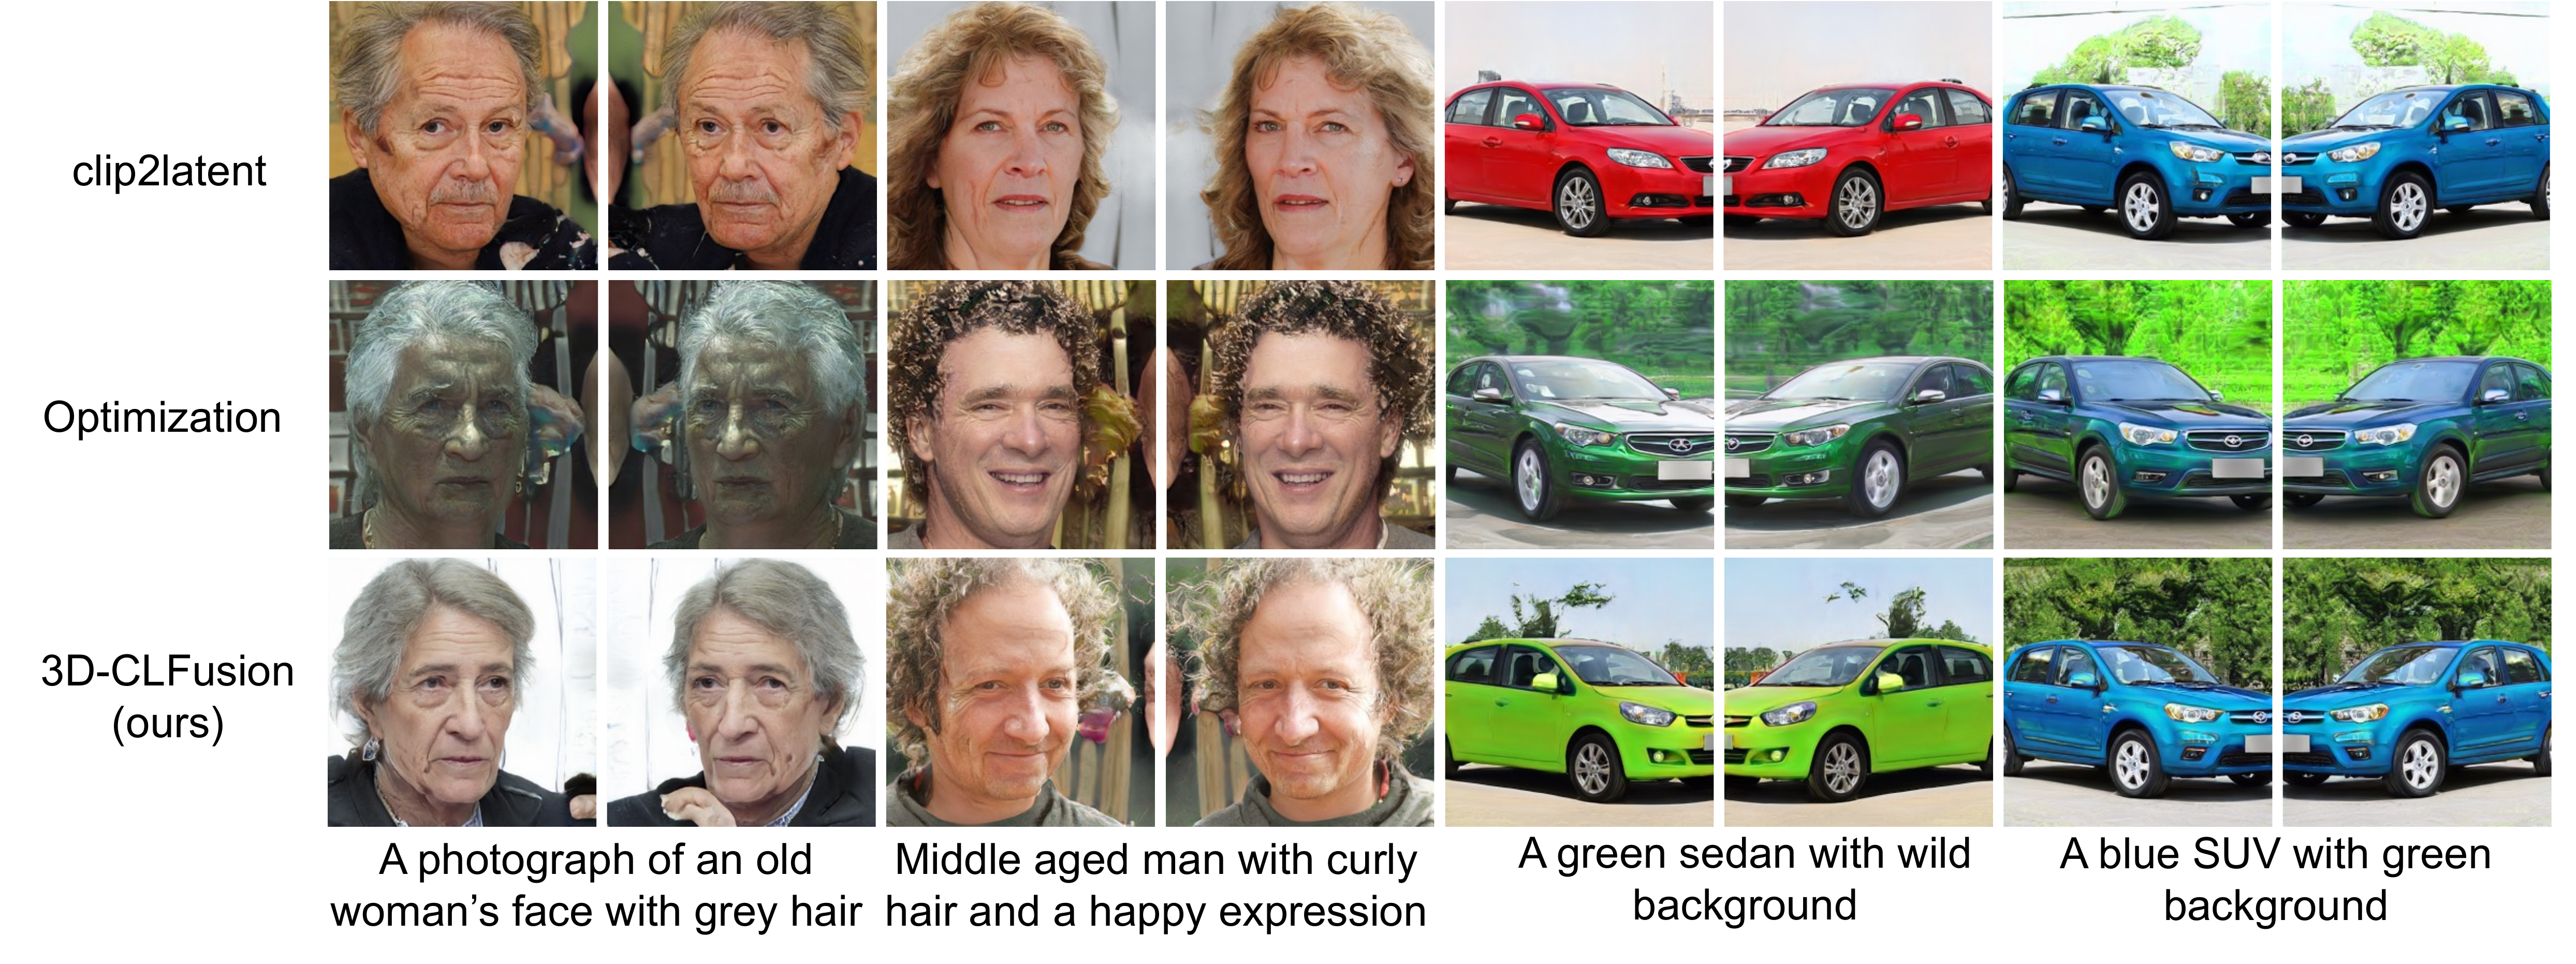}
%   \vspace{-5mm}
  \caption{Brief overview of the architecture of StyleNeRF~\cite{gu2021stylenerf}.}
  \label{fig:stylenerf}
%   \vspace{-4mm}
\end{figure}
StyleNeRF~\cite{gu2021stylenerf} has a mapping network and a synthesis network as StyleGAN~\cite{karras2019style} does. The overview of the network is roughly presented in Figure~\ref{fig:stylenerf}. For the mapping network, latent codes are sampled from standard Gaussian distribution and processed by a number of fully connected layers. The synthesis network employs
NeRF++ which consists of a unit sphere for foreground NeRF  and a background NeRF using inverted sphere parameterization. Two MLPs that represent foreground and background are used to predict the density. The color prediction is performed using another shared MLP. Each style-conditioned MLP block consists of an affine transformation layer and a 1×1 convolution layer. The convolution weights are modulated with the affine-transformed styles and then demodulated for computation. Leaky-ReLU is used as non-linear activation. We directly utilize the checkpoint provided by StyleNeRF~\cite{gu2021stylenerf} without further change on the network and the pre-trained weights. More details can be found at \cite{gu2021stylenerf}.


\paragraph{Base Encoder}
As mentioned earlier, the base encoder $E_{base}$ contains 6 residual blocks and 1 linear projection layer. The output of the encoder will be a vector of 512-dimension $w$ latent code. The network is roughly presented in Figure~\ref{fig:encoder}. Since not all of the testing data in the real world has ground truth pose from the off-the-shelf model, our base encoder can also predict the yaw and roll angles from the input image while training with the ground-truth pose outputs from the synthesized images. The output dimension will be 514 (512 plus 2) if the additional task for pose prediction is added.

\begin{figure}[t]
  \centering
  \includegraphics[width=\linewidth]{fig/encoder.pdf}
%   \vspace{-5mm}
  \caption{Brief overview of the architecture of base encoder.}
  \label{fig:encoder}
%   \vspace{-4mm}
\end{figure}

\paragraph{Residual Encoder}
The overview of the network is roughly presented in Figure~\ref{fig:pSp}.  The encoder derives the style input latent codes from three intermediate feature maps of spatial resolutions 16 × 16 (for input index 0 to 2), 32 × 32 (for input index 3 to 6), and 64 × 64 (for index 7 to last one). Each style vector is obtained from the corresponding feature map using a Map2style block, which is a convolutional network containing a series of 2-strided convolutions with LeakyReLU activations. More details can be found at \cite{richardson2021encoding}.

\begin{figure}[t]
  \centering
  \includegraphics[width=0.8\linewidth]{fig/pSp.pdf}
%   \vspace{-5mm}
  \caption{Brief overview of the architecture of residual encoder using pSp~\cite{richardson2021encoding}.}
  \label{fig:pSp}
%   \vspace{-4mm}
\end{figure}




\section{More ablation studies and results}
\label{app:abl}
% \paragraph{Synthesized images and feature-level losses.}
% To further analyze the effectiveness of using the multi-view synthesized images and the proposed feature loss $\mathcal{L}_{feat}$ ($\mathcal{L}_{feat}^{base}$ and $\mathcal{L}_{feat}^{res}$) for both base encoder and the residual encoder, we conduct the experiments each with one of them excluded. The qualitative result is presented in Figure~\ref{fig:abl}. To begin with, when the synthesized images $x_{syn}$ are excluded (note that $\mathcal{L}_{feat}$ will also be excluded without $x_{syn}$), the style latent generated by our proposed encoders are not able to preserve the reasonable face structure. The generated multi-view images have artifacts and distortion in face. In addition, if the encoders are trained with synthesized images $x_{syn}$ yet without $\mathcal{L}_{feat}$, the style latent code is able to preserve view consistency yet still has the loss of identity preservation as the full model. These studies demonstrate these two factors are significant to our model.


% \begin{figure}[t!]
%   \centering
%   \includegraphics[width=0.6\linewidth]{fig/abl.pdf}
% %   \vspace{-5mm}
%   \caption{\textbf{Ablation studies on the training images and the feature loss.}}
%   \label{fig:abl}
% %   \vspace{-4mm}
% \end{figure}

\paragraph{More qualitative results on novel rendering.}
We present more results on novel view rendering for different input images in Figure~\ref{fig:more_novel}. This figure demonstrates the generalization of our encoders plus the StyleNeRF generator to different races, gender, age, and skin tones. 

\paragraph{Generator: StyleNeRF~\cite{gu2021stylenerf} vs. EG3D~\cite{chan2022efficient}}
To analyze the significance of the generators for the NeRF inversion, we also compare the results replacing the StyleNeRF generator with Eg3D using the same input image from Figure~\ref{fig:more_novel}. EG3D~\cite{chan2022efficient} is composed of StyleGAN2 architecture and utilizes tri-plane volume rendering. More details can be referred to in their paper. We re-train the encoders using the generator EG3D~\cite{chan2022efficient} and present the results of novel-view rendering in Figure~\ref{fig:more_novel_eg3d}.

% As we see from the figure, Eg3D exhibits difficulty in the inversion of human eyes and some other details. We credit the reason for the learning of $\mathcal{W}+$ space for the triplane representation in Eg3D is not sensitive to details such as human eyes. However, even though the result of inversion is inferior to the one of StyleNeRF, it still outperform the online optimization, \textit{i.e.,} PTI~\cite{roich2021pivotal}  (see Figure~\ref{fig:eg3d_online} and the demo video). As shown from Figure~\ref{fig:eg3d_online}, our method preserves 3D structure well even though exhibits the gap from the input image. Compared with our method, PTI breaks the face structure for novel-view synthesis as well in Eg3D. However, if combining our encoder with PTI, the derived latent code is able to preserve fine details and the 3D face structure. In addition, later in the experiment on animal faces, we show that our encoders are still effective for GAN inversion of animal faces using Eg3D compared with human faces.




\section{More experiments on animal faces}\label{app:more}

To analyze the ability of our model on the inversion of animal faces, we conduct the experiments using AFHQ~\cite{choi2020starganv2}. This dataset includes three categories of animals which are cats, dogs, and wildlife. Since StyleNeRF~\cite{gu2021stylenerf} does not release the checkpoint for this dataset, we train our own checkpoint using the open-source code ourselves which may have sub-optimal rendering effectiveness. In addition, since we do not have a suitable off-the-shelf pose estimator for the animals, we additionally train the pose encoder in our base encoder (as shown in Figure~\ref{fig:encoder}) for estimating the camera pose for the animals. We present the results of NeRF inversion using our encoders in Figure~\ref{fig:afhq_novel}. In addition, we also present the NeRF inversion using the checkpoint of cat (a subset of AFHQ) released by EG3D~\cite{chan2022efficient} in Figure~\ref{fig:afhq_novel_eg3d}. These two figures show that our framework is able to perform effective 3D-aware NeRF inversion on animal faces.

\section{More experiments on stylization with CLIP}\label{app:clip}
To demonstrate the generalization of our proposed 3D-aware encoder for stylization on the $W+$ space, we utilize CLIP~\cite{radford2021learning} to further edit the produced latent from our NeRF-3DE and present the results as follows:
\begin{itemize}
    \item Stylization with the text "Zombie" (Figure~\ref{fig:zombie}).
    \item Stylization with the text "Joker" (Figure~\ref{fig:joker}).
    \item Stylization with the text "Crying face" (Figure~\ref{fig:cry}).
    \item Stylization with the text "Angry face" (Figure~\ref{fig:angry}).
    % \item Stylization with the text "Barack Obama" (Figure~\ref{fig:obama}).
    \item Stylization with the text "Albert Einstein" (Figure~\ref{fig:albert}).
\end{itemize}

\section{Code}
We implement our model using PyTorch. The source code for this paper is provided in the directory named ``Code" for review. PLEASE DO NOT DISTRIBUTE ANY SOURCE FILES. The official version will be released after acceptance.

\begin{figure*}[t]
  \centering
  \includegraphics[width=0.9\linewidth]{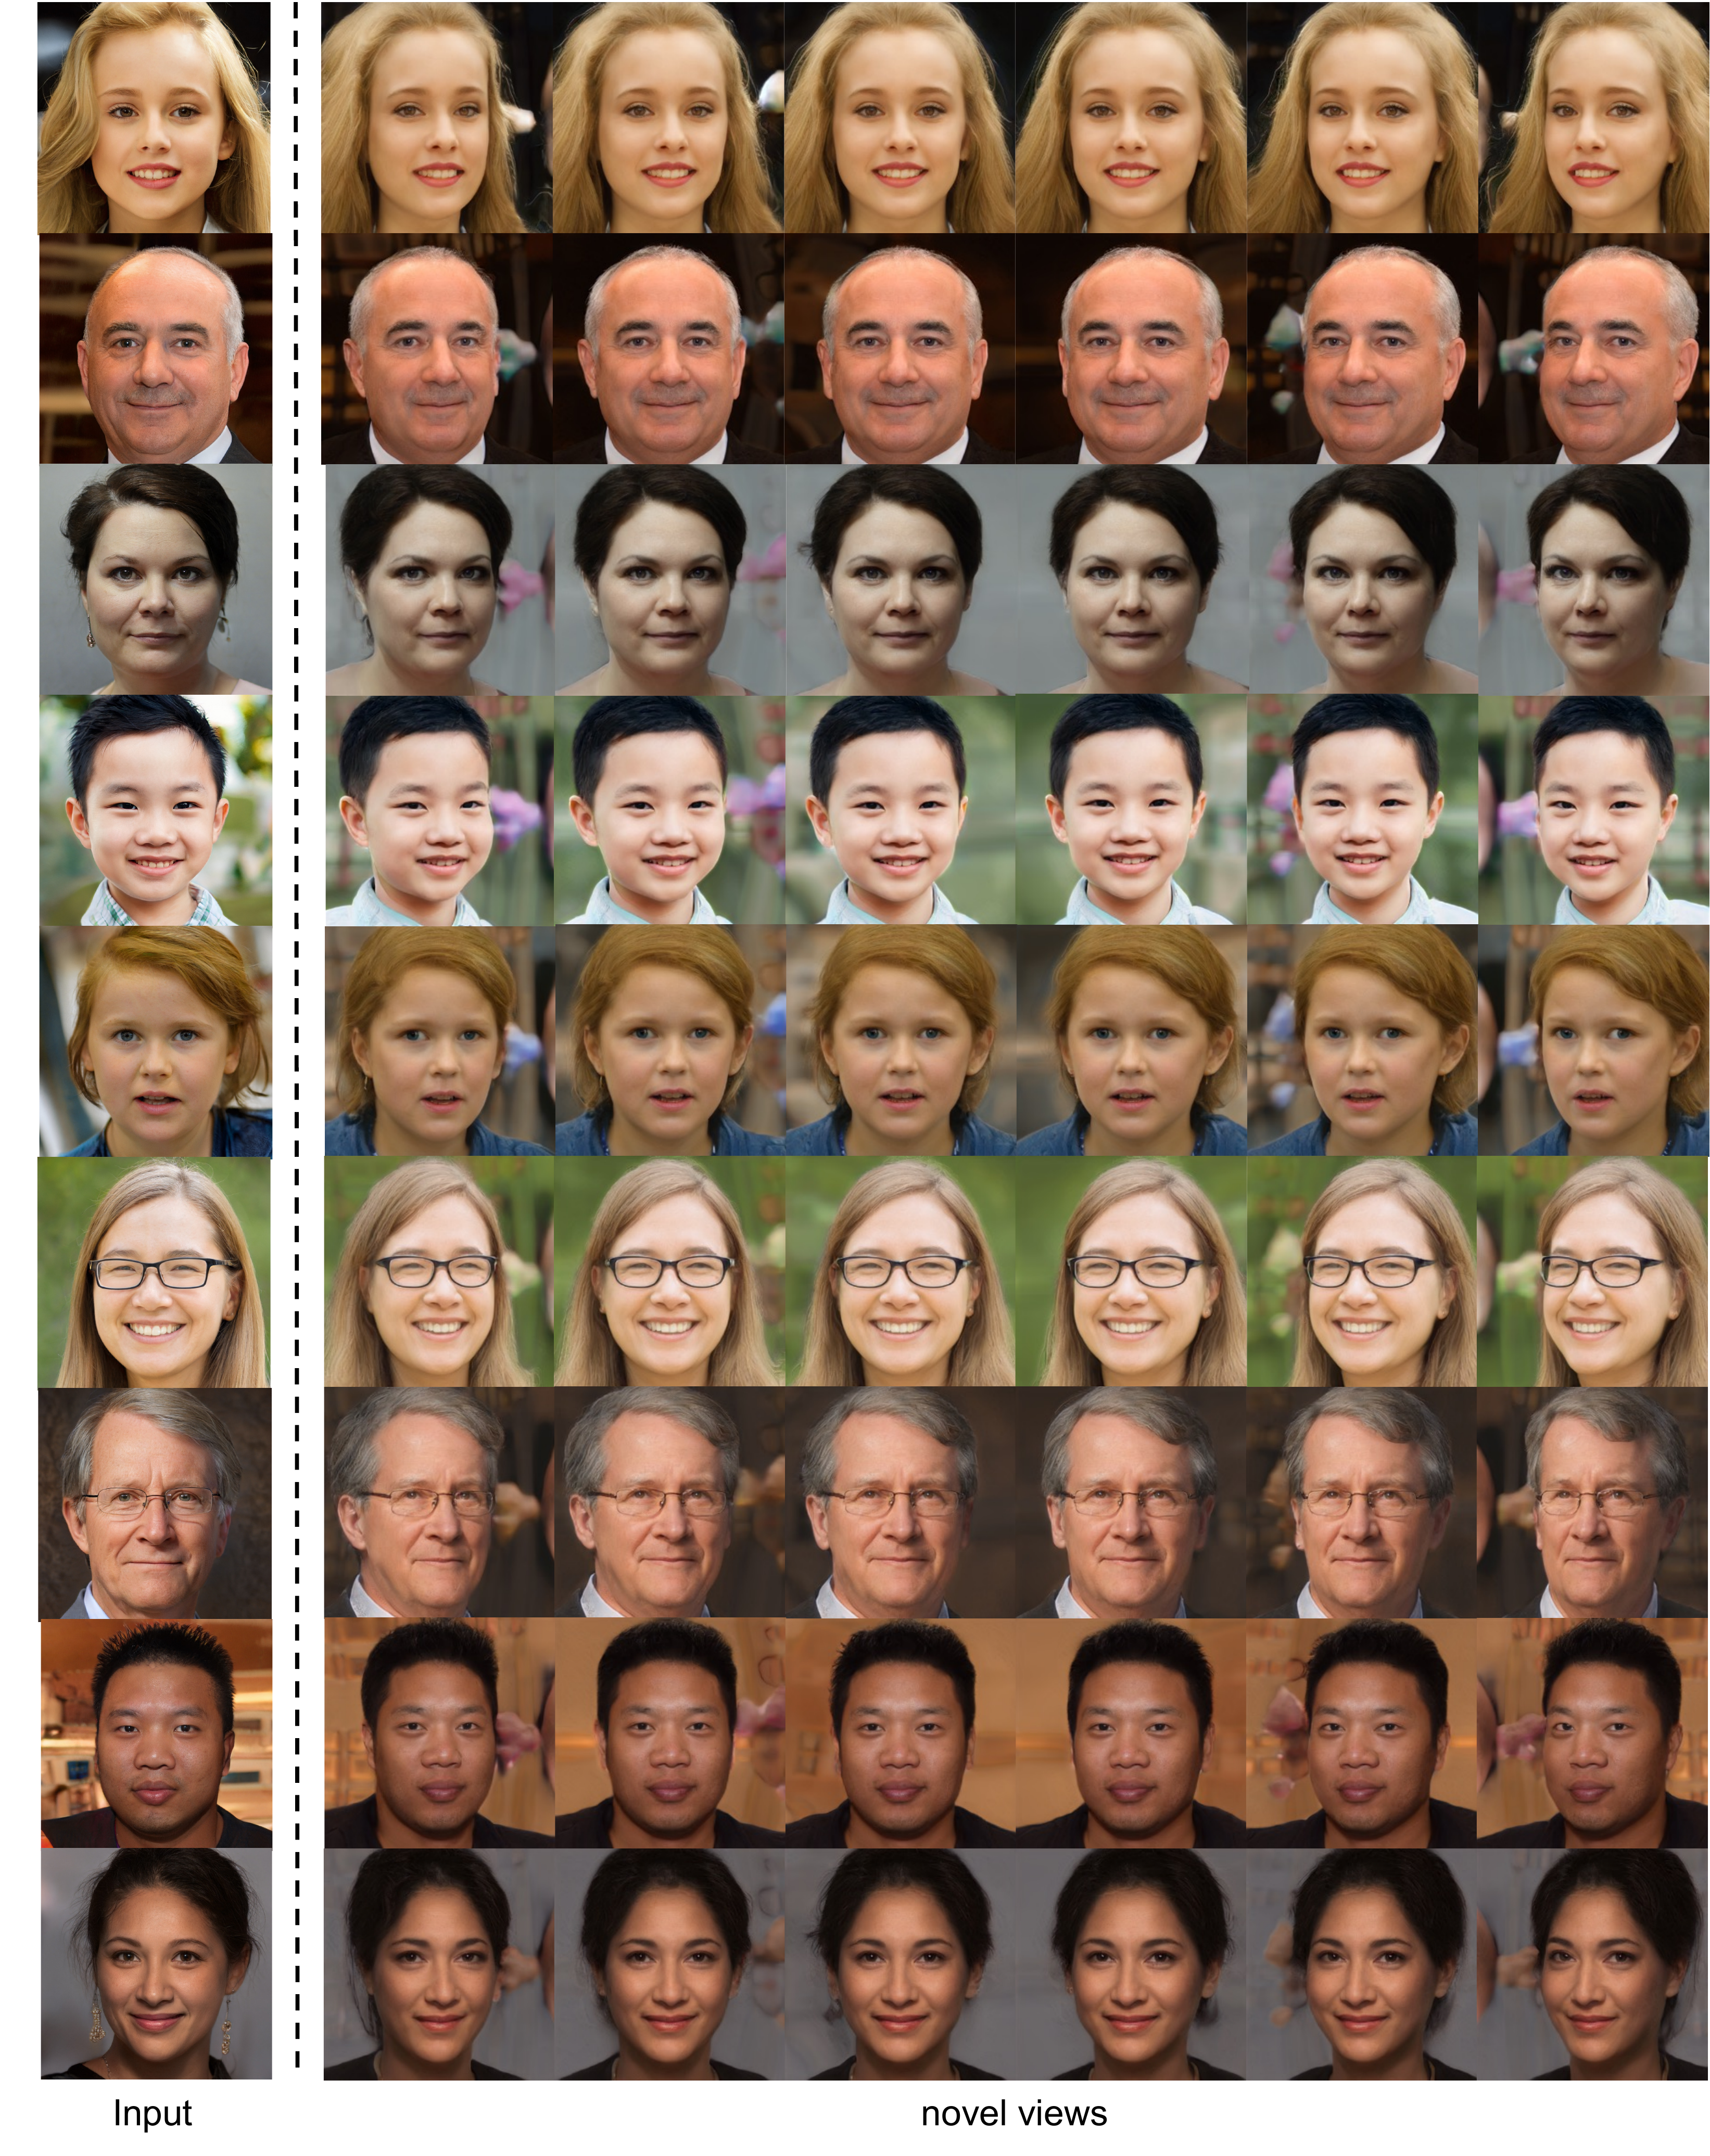}
%   \vspace{-5mm}
  \caption{{More qualitative results using our encoder for novel view rendering on StyleGAN2-Fake using StyleNeRF generator.}}
  \label{fig:more_novel}
%   \vspace{-4mm}
\end{figure*}

\begin{figure*}[t]
  \centering
  \includegraphics[width=0.9\linewidth]{fig/eg3d_pti.pdf}
%   \vspace{-5mm}
  \caption{{Results generated by combining our encoder with PTI and \textbf{Eg3D} generator for novel view rendering on StyleGAN2-Fake}.}
  \label{fig:more_novel_eg3d}
%   \vspace{-4mm}
\end{figure*}

% \begin{figure}[t]
%   \centering
%   \includegraphics[width=\linewidth]{fig/eg3d_online.pdf}
% %   \vspace{-5mm}
%   \caption{{Comparisons with online optimization (\textit{i.e.}, PTI) using our encoder for novel view rendering on StyleGAN2-Fake} replacing StyleNeRF with \textbf{Eg3D} as the generator ($\mathbf{G}$).}
%   \label{fig:eg3d_online}
% %   \vspace{-4mm}
% \end{figure}
\begin{figure*}[t]
  \centering
  \includegraphics[width=0.9\linewidth]{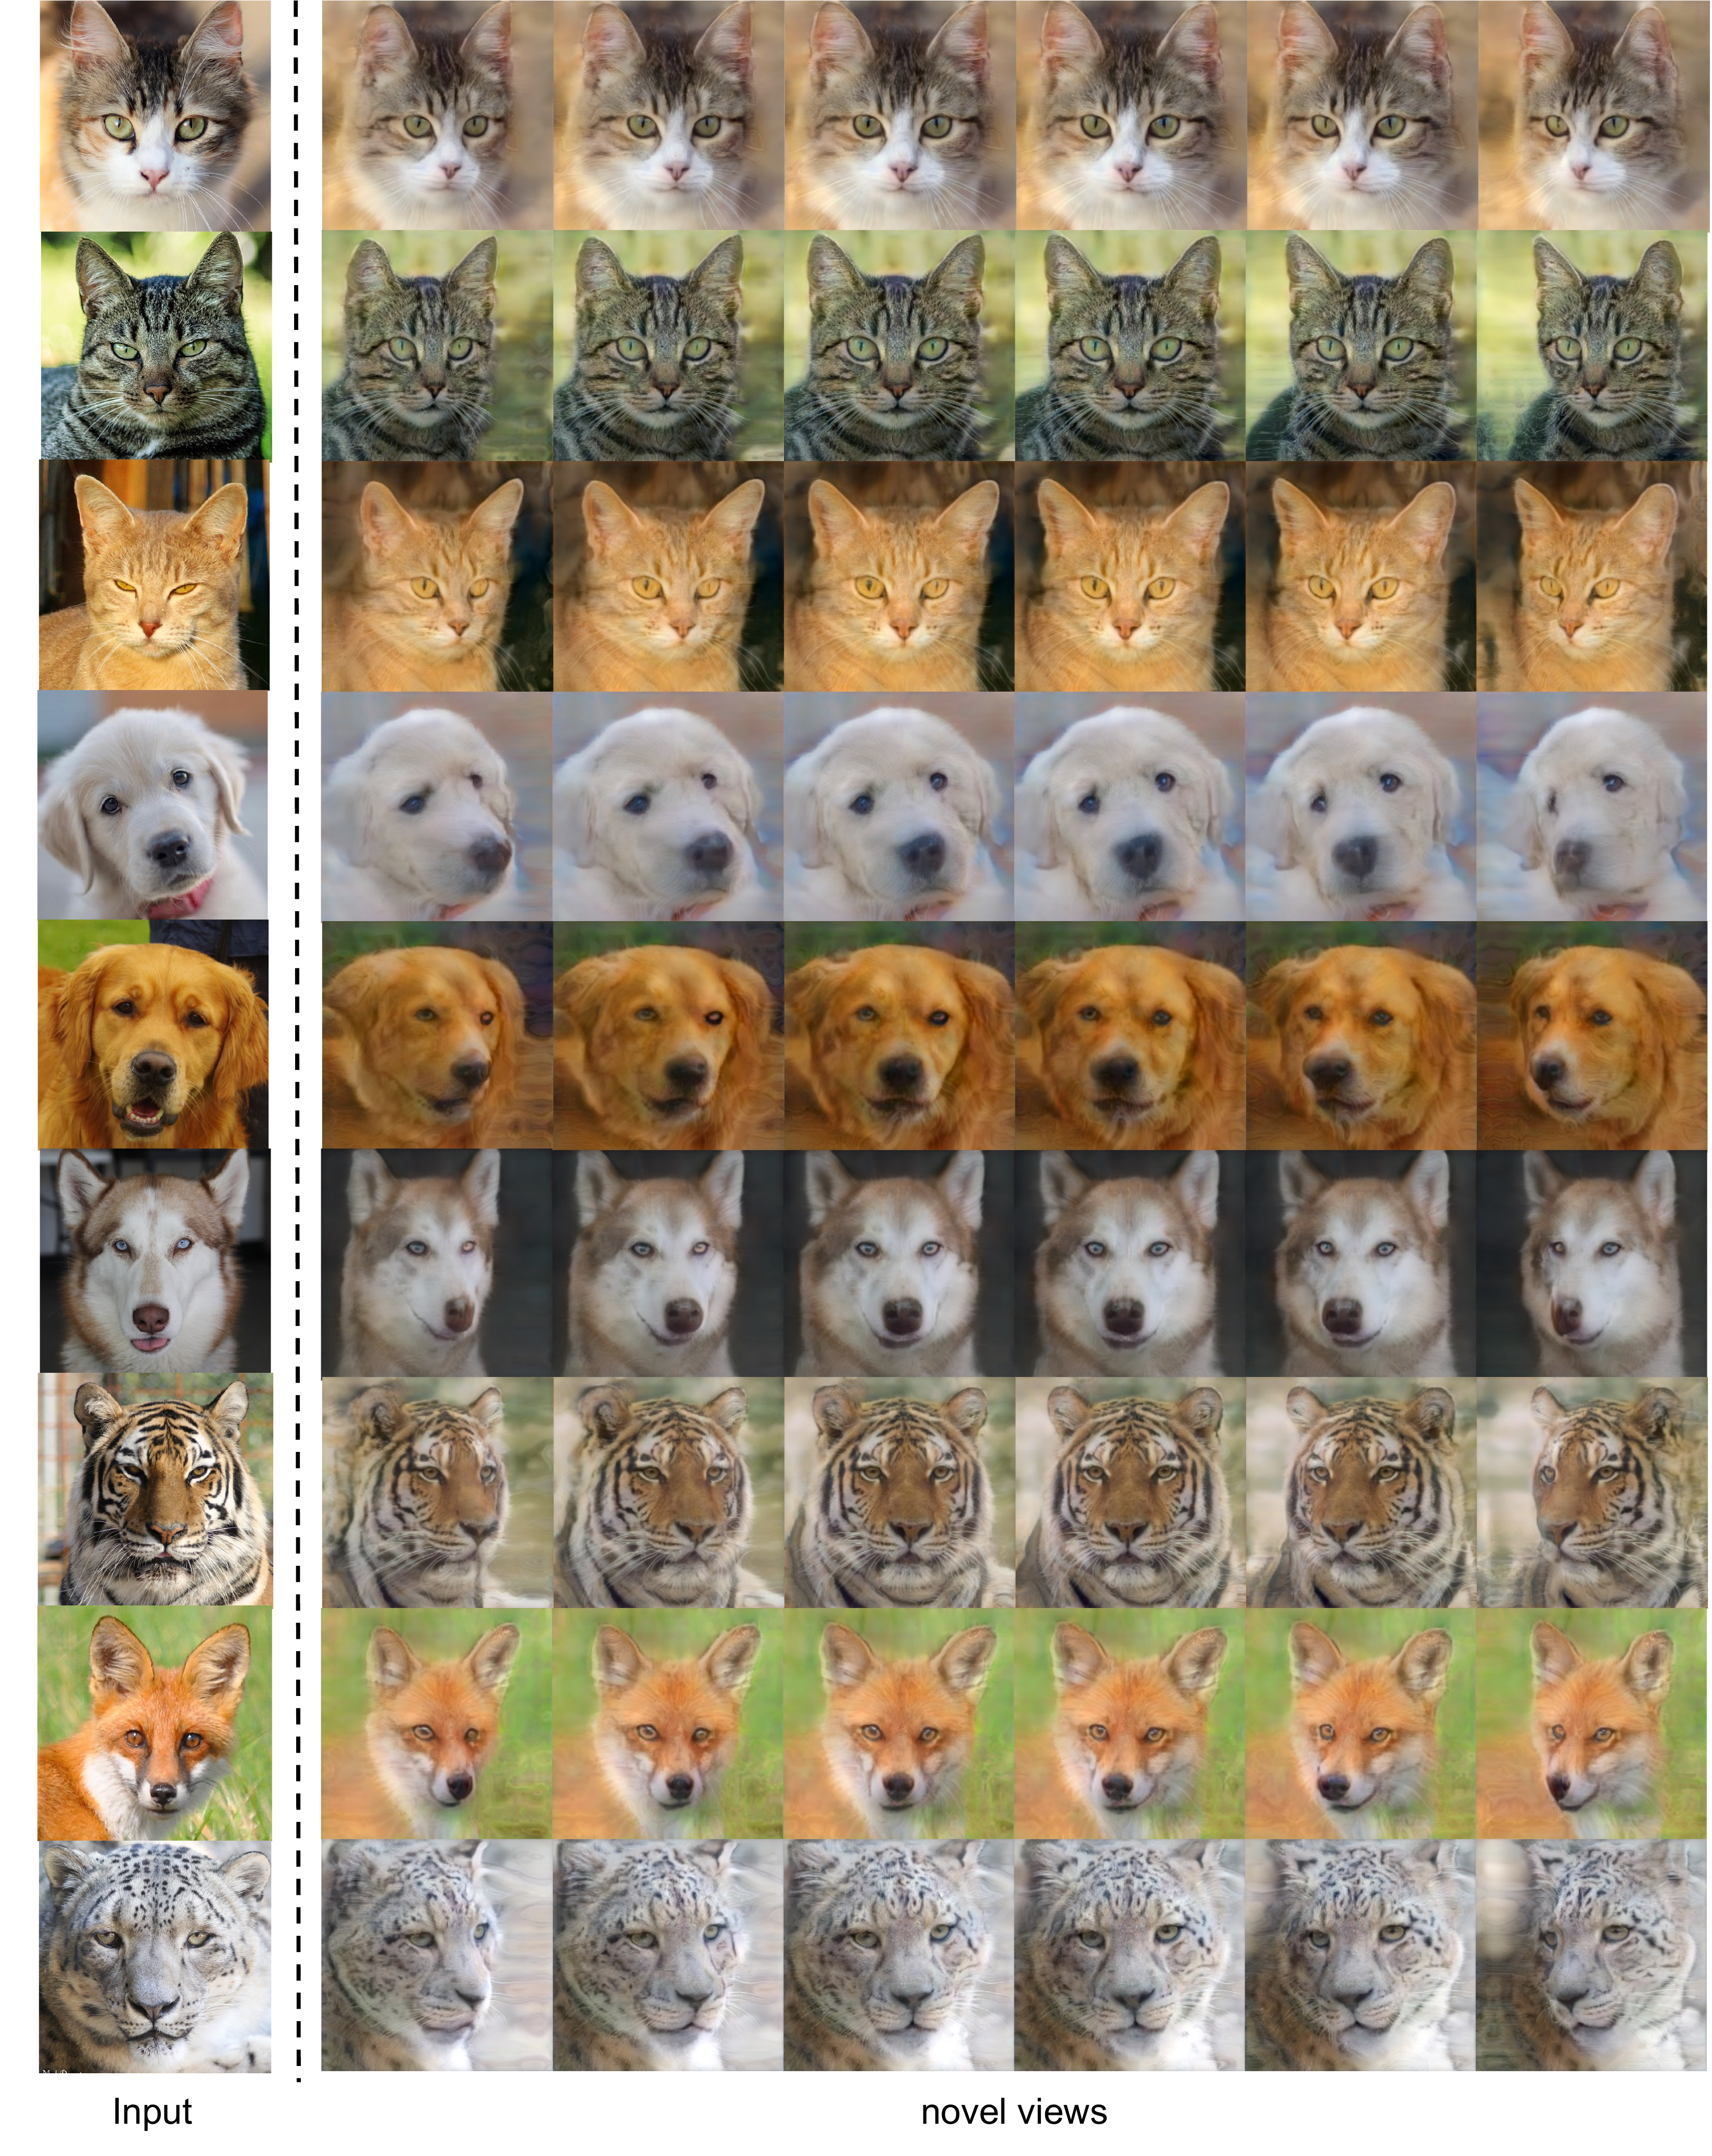}
%   \vspace{-5mm}
  \caption{Additinal qualitative results using our encoder for novel view rendering on AFHQ. Note that since the checkpoint of StyleNeRF for AFHQ is not released, we train a sup-optimal checkpoint ourselves.}
  \label{fig:afhq_novel}
%   \vspace{-4mm}
\end{figure*}

\begin{figure*}[t]
  \centering
  \includegraphics[width=0.9\linewidth]{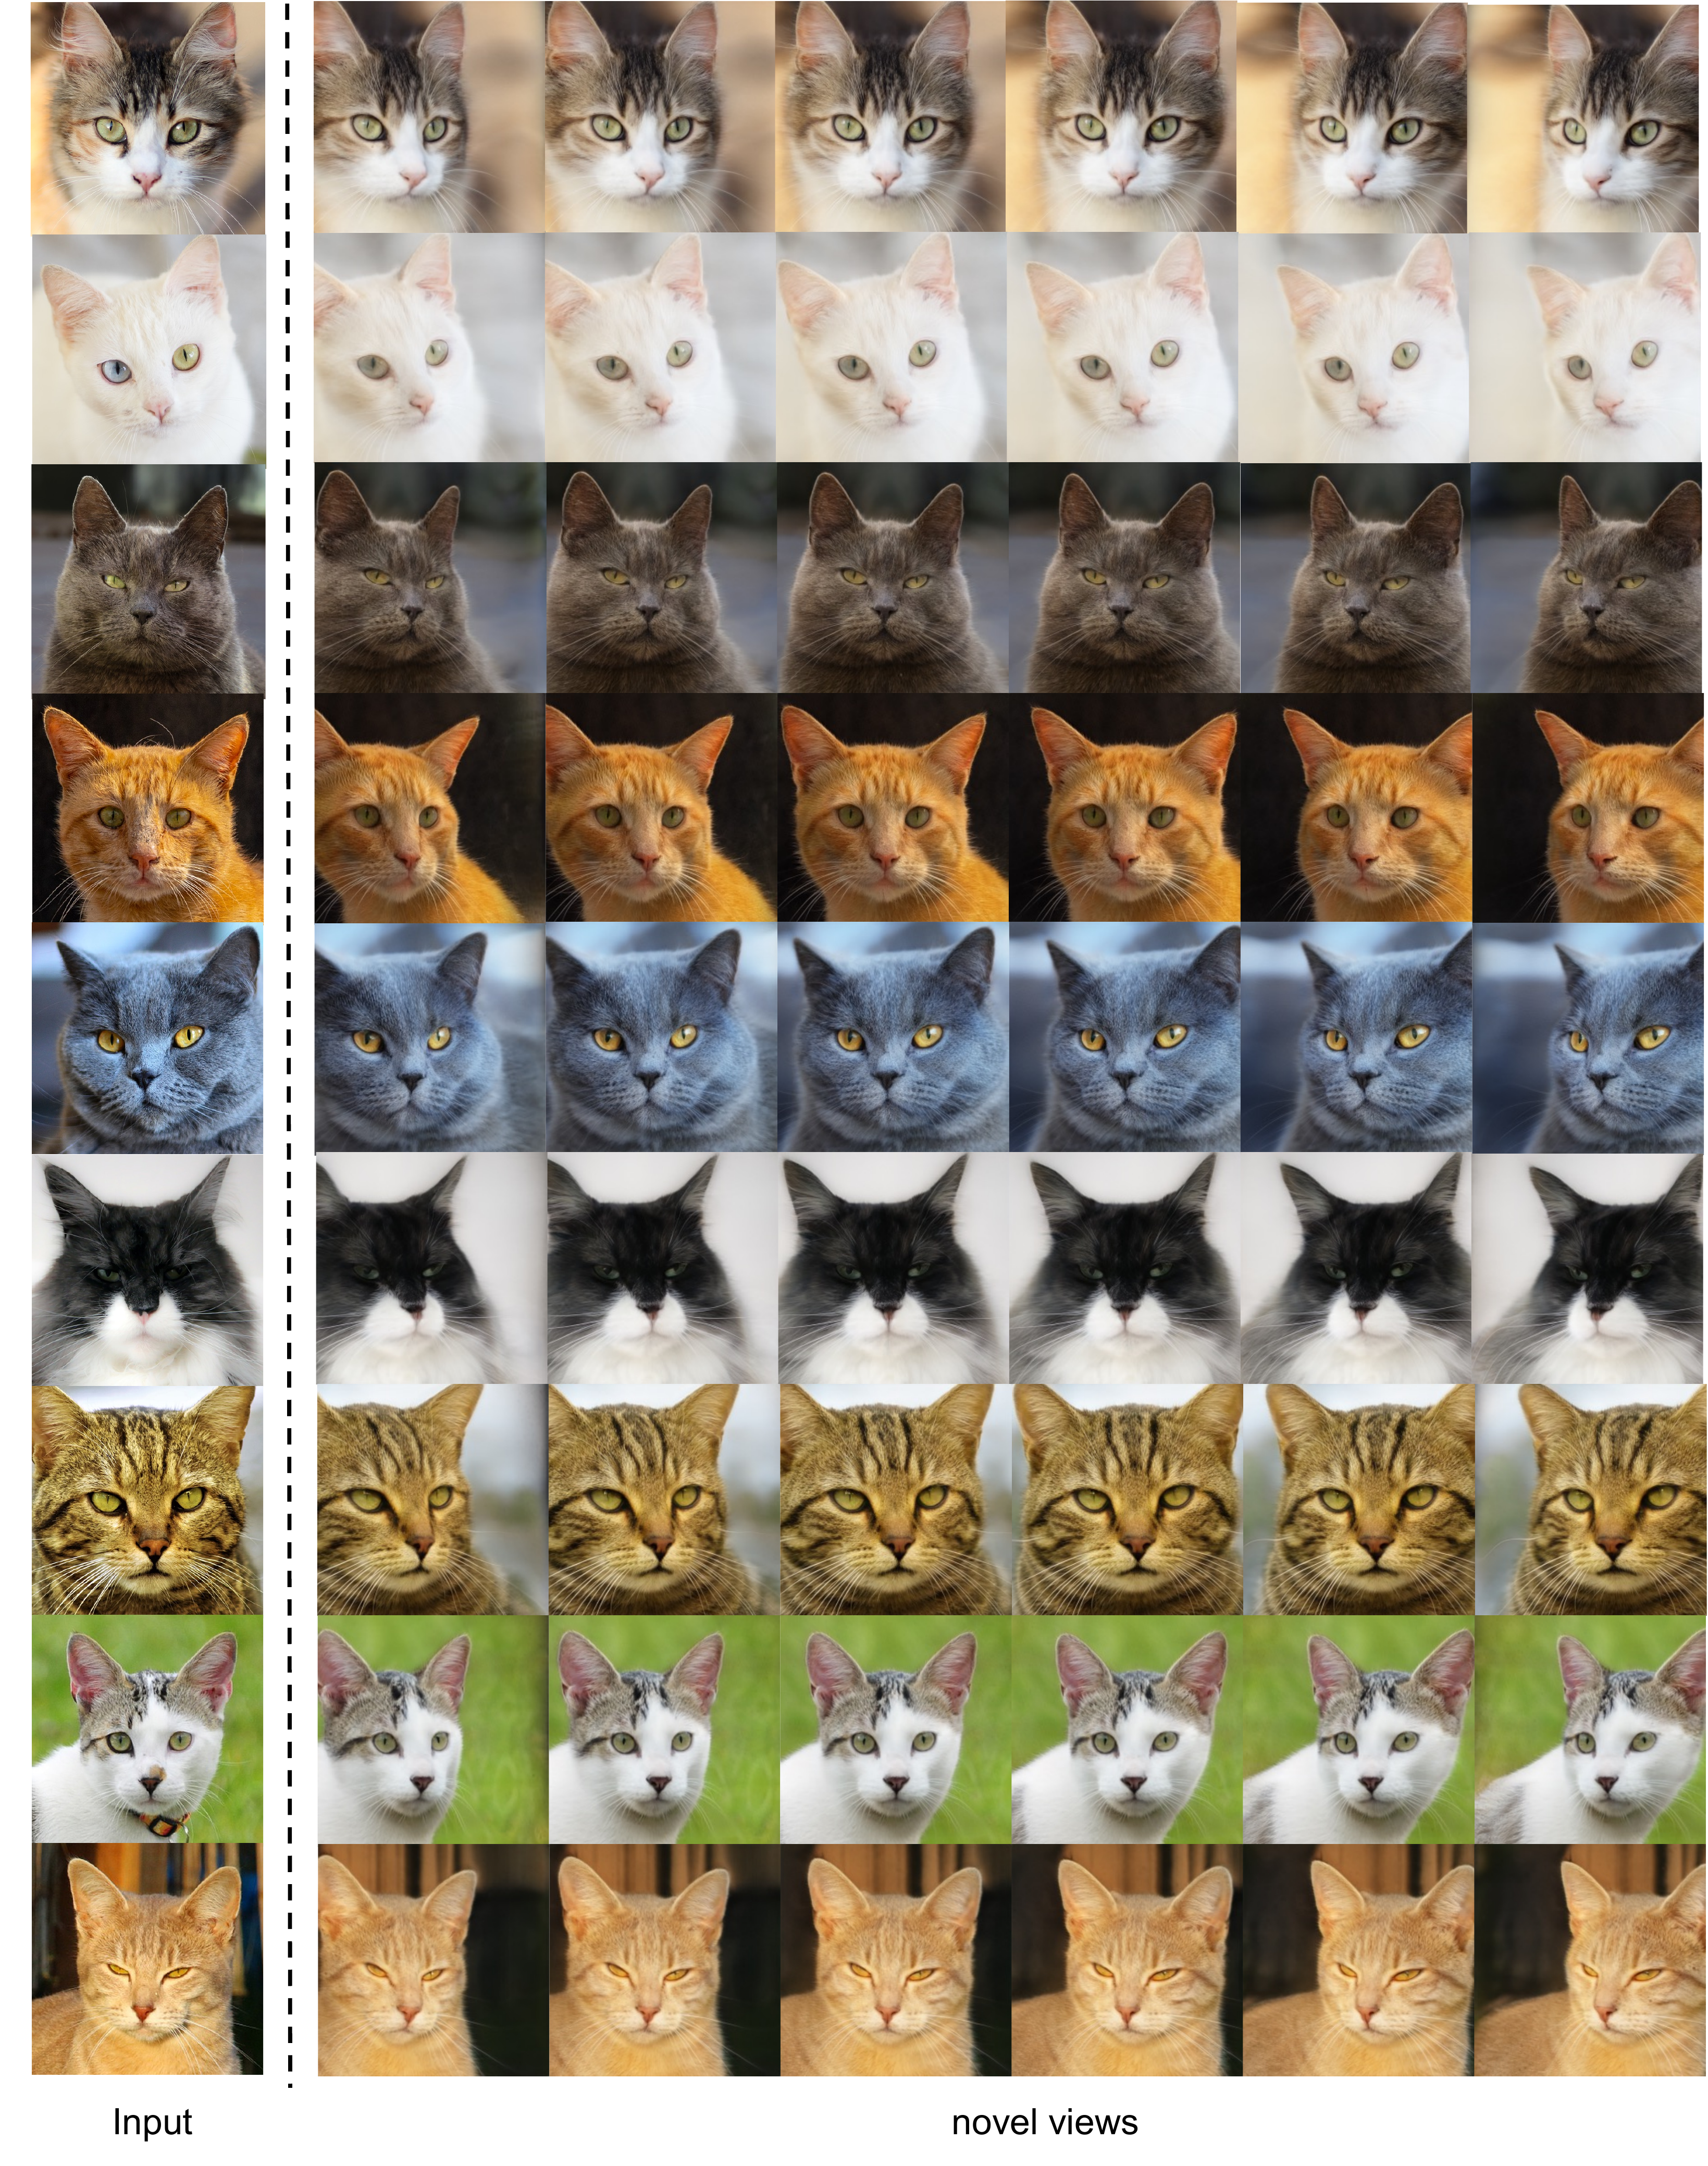}
%   \vspace{-5mm}
  \caption{Additinal qualitative results using our encoder for novel view rendering on Cats subset in AFHQ using \textbf{Eg3D} as the generator ($\mathbf{G}$).}
  \label{fig:afhq_novel_eg3d}
%   \vspace{-4mm}
\end{figure*}


\begin{figure*}[t]
  \centering
  \includegraphics[width=0.9\linewidth]{fig/zombie.pdf}
%   \vspace{-5mm}
  \caption{Stylization with the text "Zombie" using CLIP on the latent produced by our model. StyleNeRF is used as the generator.}
  \label{fig:zombie}
%   \vspace{-4mm}
\end{figure*}

\begin{figure*}[t]
  \centering
  \includegraphics[width=0.9\linewidth]{fig/joker.pdf}
%   \vspace{-5mm}
  \caption{Stylization with the text "Joker" using CLIP on the latent produced by our model. StyleNeRF is used as the generator.}
  \label{fig:joker}
%   \vspace{-4mm}
\end{figure*}

\begin{figure*}[t]
  \centering
  \includegraphics[width=0.9\linewidth]{fig/cry.pdf}
%   \vspace{-5mm}
  \caption{Stylization with the text "Crying face" using CLIP on the latent produced by our model. StyleNeRF is used as the generator.}
  \label{fig:cry}
%   \vspace{-4mm}
\end{figure*}

\begin{figure*}[t]
  \centering
  \includegraphics[width=0.9\linewidth]{fig/angry.pdf}
%   \vspace{-5mm}
  \caption{Stylization with the text "Angry face" using CLIP on the latent produced by our model. StyleNeRF is used as the generator.}
  \label{fig:angry}
%   \vspace{-4mm}
\end{figure*}


% \begin{figure*}[t]
%   \centering
%   \includegraphics[width=0.9\linewidth]{fig/obama.pdf}
% %   \vspace{-5mm}
%   \caption{Stylization with the text "Barack Obama" using CLIP on the latent produced by our model. StyleNeRF is used as the generator.}
%   \label{fig:albert}
% %   \vspace{-4mm}
% \end{figure*}

\begin{figure*}[t]
  \centering
  \includegraphics[width=0.9\linewidth]{fig/albert.pdf}
%   \vspace{-5mm}
  \caption{Stylization with the text "Albert Einstein" using CLIP on the latent produced by our model. StyleNeRF is used as the generator.}
  \label{fig:albert}
%   \vspace{-4mm}
\end{figure*}
